# Supplementary material for: ElectroChemLLM: A Multimodal LLM Pipeline for High-Fidelity Electrochemical Informatics
Source: arXiv:2611.00638 source file (2026-10-31)
Supplement: Supplementary file 1 [file appendix.tex]

\input{sections/appendix_methods}
\input{sections/appendix_results}
